# Supplementary material for: Collect-and-Distribute Transformer for 3D Point Cloud Analysis
Source: arXiv:2306.01257 source file (2023-10-31)
Supplement: Supplementary file 1 [file sec6-appendix.tex]

\clearpage
\setcounter{page}{1}
\maketitlesupplementary

In this appendix, we first analyze the point coverage concern when employing patch division (as described in~\Secref{sec:pl}). Next, we present the per-category results of CDFormer by comparing with recent state-of-the-art methods on both S3DIS and ScanNetV2. Finally, additional visualizations on the activation map and  samples from both the S3DIS and ShapeNetPart datasets are provided to qualitatively demonstrate the proposed CDFormer's effectiveness.

\section{Per-Category Results}
We additionally present per-category results for both Area 5 and 6-fold cross-validation of S3DIS, as well as the test set of ScanNetV2. Please refer to Table~\ref{tab:s3dis_area5},~\ref{tab:s3dis_cross}, and \ref{tab:scannet_perclass}.
